# Supplementary material for: Task-Driven Data Verification via Gradient Descent
Source: arXiv:1905.05843 source file (2019-05-14)
Supplement: Supplementary file 1 [file sphere_appendix.tex]

\begin{table}%{r}{0.6\textwidth}
	\begin{center}%\vspace{-4pt}
	\resizebox{0.9\textwidth}{!}{%0.8\textwidth}{!}{
			\small

			\begin{tabular}{|c|c|ccc|c||ccc|c|}
    			\hline
				\multirow{2}{*}{Dataset}   &
				\multirow{2}{*}{Method}   &
				\multicolumn{4}{|c||}{Clean validation} &
				\multicolumn{4}{|c|}{Noisy validation} \\
				\hhline{~~--------}
				&&
				Precision   &  Recall &  \hspace{10pt}F1\hspace{10pt}  & Test Accuracy &
				Precision   &  Recall &  \hspace{10pt}F1\hspace{10pt}  & Test Accuracy \\
				\hhline{|==========|}
\multirow{10}{*}{5\% noise}
&All-Train              &  $\mathbf{91.2 \pm 3.7 }$ &  $63.7 \pm 3.2$  &  $70.3 \pm 3.6$  &  $97.5 \pm 0.4$  &  $\mathbf{92.1 \pm 2.7 }$ &  $74.2 \pm 2.7$  &  $\mathbf{79.7 \pm 2.5 }$ &  $\mathbf{98.6 \pm 0.1 }$\\ \hhline{~---------}
&val-train              &  $9.0 \pm 0.3$  &  $64.8 \pm 1.3$  &  $15.7 \pm 0.5$  &  $64.4 \pm 0.6$  &  $8.6 \pm 0.2$  &  $63.5 \pm 1.0$  &  $15.1 \pm 0.4$  &  $63.5 \pm 0.7$ \\ \hhline{~---------}
&Train-End              &  $\mathbf{86.6 \pm 3.1 }$ &  $90.9 \pm 1.3$  &  $\mathbf{88.2 \pm 2.2 }$ &  $\mathbf{99.0 \pm 0.3 }$ &  $65.0 \pm 5.8$  &  $85.8 \pm 1.8$  &  $71.8 \pm 4.5$  &  $95.8 \pm 0.9$ \\ \hhline{~---------}
&Train-End no reset     &  $\mathbf{86.0 \pm 4.1 }$ &  $91.2 \pm 1.6$  &  $\mathbf{87.6 \pm 3.6 }$ &  $\mathbf{97.8 \pm 1.2 }$ &  $63.1 \pm 5.2$  &  $85.0 \pm 1.6$  &  $70.6 \pm 4.3$  &  $95.3 \pm 1.3$ \\ \hhline{~---------}
&Threshold 0.0          &  $63.0 \pm 5.9$  &  $55.6 \pm 5.0$  &  $53.3 \pm 4.2$  &  $\mathbf{98.7 \pm 0.2 }$ &  $29.2 \pm 5.3$  &  $33.1 \pm 5.5$  &  $26.7 \pm 4.0$  &  $94.0 \pm 2.1$ \\ \hhline{~---------}
&Threshold 0.0 no reset &  $50.1 \pm 4.5$  &  $65.4 \pm 4.5$  &  $52.8 \pm 4.0$  &  $\mathbf{97.9 \pm 0.9 }$ &  $32.2 \pm 5.7$  &  $42.0 \pm 5.4$  &  $29.7 \pm 3.8$  &  $95.4 \pm 1.2$ \\ \hhline{~---------}
&Threshold 0.3          &  $32.6 \pm 2.1$  &  $81.7 \pm 2.5$  &  $46.0 \pm 2.3$  &  $98.5 \pm 0.2$  &  $19.4 \pm 2.1$  &  $64.9 \pm 5.0$  &  $29.1 \pm 2.9$  &  $94.4 \pm 1.0$ \\ \hhline{~---------}
&Threshold 0.3 no reset &  $31.8 \pm 1.8$  &  $85.6 \pm 1.3$  &  $45.9 \pm 2.2$  &  $97.4 \pm 0.9$  &  $19.6 \pm 1.9$  &  $71.5 \pm 4.3$  &  $30.4 \pm 2.6$  &  $94.2 \pm 1.1$ \\ \hhline{~---------}
&Threshold 0.7          &  $25.6 \pm 1.7$  &  $90.8 \pm 1.4$  &  $39.5 \pm 2.2$  &  $98.3 \pm 0.4$  &  $16.9 \pm 1.7$  &  $81.8 \pm 3.2$  &  $27.3 \pm 2.5$  &  $88.4 \pm 3.0$ \\ \hhline{~---------}
&Threshold 0.7 no reset &  $25.8 \pm 1.4$  &  $92.0 \pm 1.6$  &  $40.0 \pm 1.8$  &  $97.3 \pm 1.0$  &  $18.4 \pm 1.6$  &  $84.1 \pm 2.0$  &  $29.7 \pm 2.2$  &  $91.2 \pm 2.4$ \\ \hhline{~---------}
&Threshold 1.0          &  $12.8 \pm 1.4$  &  $\mathbf{97.1 \pm 1.1 }$ &  $22.0 \pm 2.2$  &  $83.0 \pm 4.3$  &  $8.8 \pm 1.0$  &  $\mathbf{97.5 \pm 0.9 }$ &  $15.8 \pm 1.7$  &  $69.6 \pm 4.1$ \\ \hhline{~---------}
&Threshold 1.0 no reset &  $15.4 \pm 1.6$  &  $\mathbf{96.8 \pm 1.4 }$ &  $26.0 \pm 2.4$  &  $88.6 \pm 3.7$  &  $13.5 \pm 1.6$  &  $94.6 \pm 1.6$  &  $23.0 \pm 2.4$  &  $81.6 \pm 4.3$ \\ \hhline{~---------}
\hhline{==========}
\multirow{10}{*}{10\% noise}
&All-Train              &  $\mathbf{87.9 \pm 3.6 }$ &  $71.5 \pm 2.4$  &  $76.2 \pm 3.0$  &  $\mathbf{96.9 \pm 0.2 }$ &  $\mathbf{82.1 \pm 4.0 }$ &  $79.8 \pm 1.5$  &  $\mathbf{79.3 \pm 3.0 }$ &  $\mathbf{94.6 \pm 0.8 }$\\ \hhline{~---------}
&val-train              &  $17.7 \pm 0.4$  &  $66.3 \pm 1.0$  &  $27.9 \pm 0.6$  &  $65.5 \pm 0.6$  &  $15.5 \pm 0.4$  &  $62.5 \pm 1.0$  &  $24.8 \pm 0.6$  &  $62.2 \pm 0.5$ \\ \hhline{~---------}
&Train-End              &  $\mathbf{80.2 \pm 4.3 }$ &  $89.7 \pm 1.5$  &  $\mathbf{83.8 \pm 3.2 }$ &  $\mathbf{96.0 \pm 1.1 }$ &  $52.4 \pm 3.0$  &  $80.2 \pm 1.5$  &  $62.8 \pm 2.6$  &  $89.9 \pm 1.0$ \\ \hhline{~---------}
&Train-End no reset     &  $\mathbf{81.0 \pm 4.6 }$ &  $90.6 \pm 1.5$  &  $\mathbf{84.6 \pm 3.4 }$ &  $\mathbf{96.6 \pm 1.0 }$ &  $55.1 \pm 3.3$  &  $81.8 \pm 1.6$  &  $65.2 \pm 2.8$  &  $90.4 \pm 1.1$ \\ \hhline{~---------}
&Threshold 0.0          &  $58.7 \pm 5.9$  &  $57.9 \pm 5.1$  &  $53.5 \pm 4.8$  &  $\mathbf{95.8 \pm 0.7 }$ &  $24.0 \pm 1.9$  &  $42.2 \pm 4.4$  &  $29.3 \pm 2.4$  &  $90.0 \pm 1.6$ \\ \hhline{~---------}
&Threshold 0.0 no reset &  $60.6 \pm 5.1$  &  $60.0 \pm 5.0$  &  $56.1 \pm 4.4$  &  $\mathbf{97.0 \pm 0.6 }$ &  $27.0 \pm 2.7$  &  $46.8 \pm 4.9$  &  $32.4 \pm 3.0$  &  $90.6 \pm 1.6$ \\ \hhline{~---------}
&Threshold 0.3          &  $46.5 \pm 3.8$  &  $84.6 \pm 1.7$  &  $58.4 \pm 3.3$  &  $\mathbf{95.7 \pm 0.9 }$ &  $23.2 \pm 1.3$  &  $70.3 \pm 3.6$  &  $34.7 \pm 1.9$  &  $89.3 \pm 0.9$ \\ \hhline{~---------}
&Threshold 0.3 no reset &  $45.6 \pm 3.6$  &  $86.8 \pm 1.5$  &  $58.4 \pm 3.5$  &  $\mathbf{95.9 \pm 0.8 }$ &  $27.1 \pm 1.8$  &  $75.8 \pm 1.5$  &  $39.2 \pm 1.9$  &  $89.3 \pm 1.1$ \\ \hhline{~---------}
&Threshold 0.7          &  $39.0 \pm 2.6$  &  $92.2 \pm 1.2$  &  $53.9 \pm 2.7$  &  $\mathbf{96.2 \pm 1.0 }$ &  $21.8 \pm 1.1$  &  $80.5 \pm 2.5$  &  $34.2 \pm 1.5$  &  $87.6 \pm 1.4$ \\ \hhline{~---------}
&Threshold 0.7 no reset &  $40.1 \pm 3.1$  &  $92.5 \pm 1.4$  &  $54.8 \pm 3.3$  &  $\mathbf{96.8 \pm 0.8 }$ &  $24.4 \pm 1.7$  &  $85.0 \pm 1.4$  &  $37.4 \pm 1.9$  &  $86.7 \pm 1.3$ \\ \hhline{~---------}
&Threshold 1.0          &  $24.2 \pm 2.3$  &  $\mathbf{97.5 \pm 0.9 }$ &  $37.6 \pm 3.0$  &  $82.5 \pm 4.2$  &  $15.0 \pm 0.7$  &  $\mathbf{93.4 \pm 1.2 }$ &  $25.7 \pm 1.0$  &  $72.5 \pm 2.3$ \\ \hhline{~---------}
&Threshold 1.0 no reset &  $25.6 \pm 2.6$  &  $\mathbf{97.2 \pm 0.9 }$ &  $39.3 \pm 3.3$  &  $83.4 \pm 4.5$  &  $18.1 \pm 1.5$  &  $\mathbf{94.7 \pm 1.2 }$ &  $29.7 \pm 2.1$  &  $74.8 \pm 3.3$ \\ \hhline{~---------}
\hhline{==========}
\multirow{10}{*}{20\% noise}
&All-Train              &  $\mathbf{88.5 \pm 1.8 }$ &  $76.5 \pm 1.2$  &  $81.7 \pm 1.3$  &  $91.8 \pm 0.6$  &  $\mathbf{84.3 \pm 2.8 }$ &  $75.4 \pm 1.3$  &  $\mathbf{78.9 \pm 2.0 }$ &  $\mathbf{91.2 \pm 0.7 }$\\ \hhline{~---------}
&val-train              &  $33.4 \pm 0.6$  &  $66.8 \pm 0.7$  &  $44.5 \pm 0.7$  &  $66.8 \pm 0.7$  &  $25.2 \pm 0.5$  &  $57.4 \pm 0.8$  &  $35.0 \pm 0.6$  &  $57.8 \pm 0.6$ \\ \hhline{~---------}
&Train-End              &  $\mathbf{84.7 \pm 2.1 }$ &  $89.1 \pm 1.1$  &  $\mathbf{86.7 \pm 1.6 }$ &  $\mathbf{94.6 \pm 0.7 }$ &  $46.3 \pm 2.0$  &  $72.7 \pm 1.4$  &  $56.4 \pm 1.9$  &  $76.7 \pm 1.3$ \\ \hhline{~---------}
&Train-End no reset     &  $84.5 \pm 2.1$  &  $89.4 \pm 0.7$  &  $\mathbf{86.7 \pm 1.4 }$ &  $\mathbf{94.7 \pm 0.8 }$ &  $46.2 \pm 2.0$  &  $71.2 \pm 1.3$  &  $55.8 \pm 1.8$  &  $77.3 \pm 1.1$ \\ \hhline{~---------}
&Threshold 0.0          &  $69.7 \pm 3.5$  &  $53.1 \pm 5.1$  &  $56.9 \pm 4.4$  &  $92.4 \pm 0.8$  &  $34.3 \pm 0.9$  &  $56.8 \pm 2.1$  &  $42.4 \pm 1.1$  &  $77.3 \pm 1.3$ \\ \hhline{~---------}
&Threshold 0.0 no reset &  $63.7 \pm 3.2$  &  $49.4 \pm 5.8$  &  $52.1 \pm 4.9$  &  $88.8 \pm 2.4$  &  $34.9 \pm 0.9$  &  $57.6 \pm 1.7$  &  $43.2 \pm 0.9$  &  $78.6 \pm 1.2$ \\ \hhline{~---------}
&Threshold 0.3          &  $61.6 \pm 1.9$  &  $84.6 \pm 1.6$  &  $71.1 \pm 1.7$  &  $\mathbf{93.3 \pm 0.7 }$ &  $33.8 \pm 0.8$  &  $69.3 \pm 1.3$  &  $45.3 \pm 0.9$  &  $76.3 \pm 1.2$ \\ \hhline{~---------}
&Threshold 0.3 no reset &  $59.9 \pm 1.3$  &  $84.3 \pm 1.5$  &  $69.8 \pm 1.2$  &  $\mathbf{93.8 \pm 0.7 }$ &  $33.7 \pm 0.7$  &  $69.8 \pm 1.3$  &  $45.4 \pm 0.8$  &  $77.1 \pm 1.0$ \\ \hhline{~---------}
&Threshold 0.7          &  $56.3 \pm 1.9$  &  $90.1 \pm 1.1$  &  $69.1 \pm 1.7$  &  $\mathbf{93.3 \pm 0.8 }$ &  $33.1 \pm 0.8$  &  $75.3 \pm 1.3$  &  $46.0 \pm 0.9$  &  $74.6 \pm 1.2$ \\ \hhline{~---------}
&Threshold 0.7 no reset &  $54.9 \pm 1.2$  &  $90.4 \pm 1.0$  &  $68.2 \pm 1.1$  &  $\mathbf{94.3 \pm 0.8 }$ &  $33.1 \pm 0.7$  &  $74.8 \pm 1.3$  &  $45.8 \pm 0.8$  &  $75.7 \pm 1.1$ \\ \hhline{~---------}
&Threshold 1.0          &  $37.7 \pm 2.7$  &  $\mathbf{97.7 \pm 0.6 }$ &  $53.1 \pm 2.8$  &  $85.5 \pm 3.1$  &  $31.5 \pm 0.9$  &  $\mathbf{81.8 \pm 1.6 }$ &  $45.3 \pm 1.0$  &  $72.6 \pm 1.2$ \\ \hhline{~---------}
&Threshold 1.0 no reset &  $36.1 \pm 2.4$  &  $\mathbf{97.3 \pm 0.4 }$ &  $51.7 \pm 2.7$  &  $82.3 \pm 4.0$  &  $30.8 \pm 0.6$  &  $\mathbf{82.2 \pm 1.6 }$ &  $44.6 \pm 0.7$  &  $72.9 \pm 1.4$ \\ \hhline{~---------}
\hhline{==========}
\multirow{10}{*}{40\% noise}
&All-Train              &  $68.7 \pm 1.2$  &  $47.2 \pm 1.8$  &  $55.4 \pm 1.7$  &  $67.9 \pm 0.5$  &  $\mathbf{60.2 \pm 1.4 }$ &  $40.7 \pm 1.7$  &  $47.9 \pm 1.5$  &  $\mathbf{64.3 \pm 0.7 }$\\ \hhline{~---------}
&val-train              &  $57.4 \pm 0.8$  &  $67.2 \pm 0.8$  &  $61.9 \pm 0.8$  &  $66.8 \pm 0.7$  &  $43.1 \pm 0.6$  &  $52.9 \pm 0.7$  &  $47.5 \pm 0.6$  &  $52.5 \pm 0.5$ \\ \hhline{~---------}
&Train-End              &  $\mathbf{78.2 \pm 1.7 }$ &  $78.1 \pm 1.1$  &  $\mathbf{78.1 \pm 1.3 }$ &  $\mathbf{81.7 \pm 1.2 }$ &  $49.1 \pm 0.8$  &  $56.9 \pm 1.2$  &  $\mathbf{52.7 \pm 1.0 }$ &  $58.4 \pm 0.8$ \\ \hhline{~---------}
&Train-End no reset     &  $\mathbf{75.2 \pm 2.0 }$ &  $77.1 \pm 1.4$  &  $\mathbf{76.1 \pm 1.7 }$ &  $\mathbf{79.5 \pm 1.5 }$ &  $49.6 \pm 1.2$  &  $56.4 \pm 1.1$  &  $\mathbf{52.8 \pm 1.1 }$ &  $59.0 \pm 1.0$ \\ \hhline{~---------}
&Threshold 0.0          &  $\mathbf{75.9 \pm 2.0 }$ &  $55.7 \pm 3.4$  &  $62.2 \pm 2.1$  &  $78.0 \pm 0.7$  &  $45.9 \pm 0.7$  &  $51.3 \pm 1.0$  &  $48.4 \pm 0.8$  &  $58.7 \pm 0.9$ \\ \hhline{~---------}
&Threshold 0.0 no reset &  $73.4 \pm 1.8$  &  $64.8 \pm 2.7$  &  $67.6 \pm 1.7$  &  $78.2 \pm 0.9$  &  $46.8 \pm 1.0$  &  $50.4 \pm 1.0$  &  $48.5 \pm 0.9$  &  $59.5 \pm 0.8$ \\ \hhline{~---------}
&Threshold 0.3          &  $72.8 \pm 1.4$  &  $77.5 \pm 0.7$  &  $75.0 \pm 0.9$  &  $\mathbf{80.5 \pm 1.0 }$ &  $45.7 \pm 0.6$  &  $58.5 \pm 1.1$  &  $51.3 \pm 0.8$  &  $58.4 \pm 0.8$ \\ \hhline{~---------}
&Threshold 0.3 no reset &  $70.7 \pm 1.5$  &  $78.7 \pm 0.9$  &  $74.4 \pm 1.1$  &  $\mathbf{79.5 \pm 1.2 }$ &  $46.4 \pm 0.8$  &  $57.6 \pm 1.1$  &  $51.4 \pm 0.9$  &  $59.2 \pm 0.8$ \\ \hhline{~---------}
&Threshold 0.7          &  $70.8 \pm 1.2$  &  $82.0 \pm 0.9$  &  $\mathbf{75.9 \pm 1.0 }$ &  $\mathbf{80.9 \pm 1.1 }$ &  $45.6 \pm 0.6$  &  $62.1 \pm 1.2$  &  $\mathbf{52.6 \pm 0.7 }$ &  $58.5 \pm 0.9$ \\ \hhline{~---------}
&Threshold 0.7 no reset &  $69.1 \pm 1.3$  &  $82.0 \pm 1.1$  &  $75.0 \pm 1.2$  &  $\mathbf{79.8 \pm 1.3 }$ &  $46.0 \pm 0.8$  &  $61.0 \pm 1.2$  &  $\mathbf{52.5 \pm 0.9 }$ &  $58.2 \pm 0.8$ \\ \hhline{~---------}
&Threshold 1.0          &  $62.9 \pm 1.3$  &  $\mathbf{87.7 \pm 1.3 }$ &  $73.0 \pm 0.9$  &  $\mathbf{80.2 \pm 1.1 }$ &  $45.1 \pm 0.5$  &  $\mathbf{65.8 \pm 1.3 }$ &  $\mathbf{53.5 \pm 0.8 }$ &  $57.1 \pm 0.7$ \\ \hhline{~---------}
&Threshold 1.0 no reset &  $63.9 \pm 1.0$  &  $\mathbf{85.8 \pm 1.4 }$ &  $73.1 \pm 0.9$  &  $78.4 \pm 1.3$  &  $45.6 \pm 0.8$  &  $\mathbf{65.0 \pm 1.3 }$ &  $\mathbf{53.6 \pm 1.0 }$ &  $58.0 \pm 0.8$ \\ \hhline{~---------}
\hhline{==========}
\multirow{10}{*}{70\% noise}
&All-Train              &  $72.0 \pm 1.4$  &  $46.6 \pm 1.5$  &  $56.4 \pm 1.5$  &  $55.1 \pm 0.7$   &    -----      &    -----      &    -----      &    -----    \\ \hhline{~---------}
&val-train              &  $81.8 \pm 0.5$  &  $65.4 \pm 0.8$  &  $72.7 \pm 0.7$  &  $66.0 \pm 0.7$   &    -----      &    -----      &    -----      &    -----    \\ \hhline{~---------}
&Train-End              &  $84.2 \pm 0.6$  &  $64.2 \pm 1.1$  &  $72.8 \pm 0.9$  &  $66.0 \pm 0.9$   &    -----      &    -----      &    -----      &    -----    \\ \hhline{~---------}
&Train-End no reset     &  $84.3 \pm 0.5$  &  $65.7 \pm 0.8$  &  $73.8 \pm 0.6$  &  $\mathbf{67.1 \pm 0.8 }$  &    -----      &    -----      &    -----      &    -----    \\ \hhline{~---------}
&Threshold 0.0          &  $\mathbf{88.8 \pm 0.5 }$ &  $69.6 \pm 1.0$  &  $78.0 \pm 0.7$  &  $66.2 \pm 1.0$   &    -----      &    -----      &    -----      &    -----    \\ \hhline{~---------}
&Threshold 0.0 no reset &  $\mathbf{88.8 \pm 0.5 }$ &  $70.6 \pm 0.6$  &  $78.6 \pm 0.5$  &  $\mathbf{67.6 \pm 0.7 }$  &    -----      &    -----      &    -----      &    -----    \\ \hhline{~---------}
&Threshold 0.3          &  $87.6 \pm 0.5$  &  $74.5 \pm 1.0$  &  $80.5 \pm 0.7$  &  $\mathbf{67.7 \pm 1.0 }$  &    -----      &    -----      &    -----      &    -----    \\ \hhline{~---------}
&Threshold 0.3 no reset &  $87.6 \pm 0.5$  &  $75.7 \pm 0.7$  &  $81.2 \pm 0.5$  &  $\mathbf{68.4 \pm 0.9 }$  &    -----      &    -----      &    -----      &    -----    \\ \hhline{~---------}
&Threshold 0.7          &  $86.6 \pm 0.5$  &  $76.8 \pm 1.0$  &  $81.4 \pm 0.7$  &  $\mathbf{67.1 \pm 1.0 }$  &    -----      &    -----      &    -----      &    -----    \\ \hhline{~---------}
&Threshold 0.7 no reset &  $86.6 \pm 0.4$  &  $78.2 \pm 0.7$  &  $\mathbf{82.2 \pm 0.5 }$ &  $\mathbf{67.5 \pm 1.0 }$  &    -----      &    -----      &    -----      &    -----    \\ \hhline{~---------}
&Threshold 1.0          &  $85.3 \pm 0.5$  &  $\mathbf{79.2 \pm 1.0 }$ &  $\mathbf{82.1 \pm 0.7 }$ &  $66.1 \pm 1.2$   &    -----      &    -----      &    -----      &    -----    \\ \hhline{~---------}
&Threshold 1.0 no reset &  $85.3 \pm 0.4$  &  $\mathbf{80.6 \pm 0.7 }$ &  $\mathbf{82.9 \pm 0.5 }$ &  $66.5 \pm 0.9$   &    -----      &    -----      &    -----      &    -----    \\ \hhline{~---------}
\hhline{==========}
\multirow{10}{*}{90\% noise}
&All-Train              &  $89.2 \pm 0.4$  &  $46.8 \pm 0.9$  &  $61.3 \pm 0.8$  &  $49.1 \pm 0.5$   &    -----      &    -----      &    -----      &    -----    \\ \hhline{~---------}
&val-train              &  $94.8 \pm 0.2$  &  $66.1 \pm 0.8$  &  $77.8 \pm 0.6$  &  $\mathbf{66.2 \pm 0.8 }$  &    -----      &    -----      &    -----      &    -----    \\ \hhline{~---------}
&Train-End              &  $91.7 \pm 0.4$  &  $51.4 \pm 0.7$  &  $65.9 \pm 0.6$  &  $52.6 \pm 0.5$   &    -----      &    -----      &    -----      &    -----    \\ \hhline{~---------}
&Train-End no reset     &  $91.5 \pm 0.2$  &  $52.1 \pm 0.5$  &  $66.4 \pm 0.5$  &  $52.5 \pm 0.6$   &    -----      &    -----      &    -----      &    -----    \\ \hhline{~---------}
&Threshold 0.0          &  $\mathbf{96.3 \pm 0.3 }$ &  $64.4 \pm 1.0$  &  $77.1 \pm 0.8$  &  $46.5 \pm 0.8$   &    -----      &    -----      &    -----      &    -----    \\ \hhline{~---------}
&Threshold 0.0 no reset &  $\mathbf{96.7 \pm 0.2 }$ &  $66.7 \pm 1.0$  &  $78.8 \pm 0.8$  &  $47.4 \pm 0.9$   &    -----      &    -----      &    -----      &    -----    \\ \hhline{~---------}
&Threshold 0.3          &  $95.8 \pm 0.3$  &  $70.7 \pm 1.1$  &  $81.3 \pm 0.8$  &  $50.7 \pm 0.9$   &    -----      &    -----      &    -----      &    -----    \\ \hhline{~---------}
&Threshold 0.3 no reset &  $96.1 \pm 0.2$  &  $73.2 \pm 0.9$  &  $83.1 \pm 0.7$  &  $50.8 \pm 0.8$   &    -----      &    -----      &    -----      &    -----    \\ \hhline{~---------}
&Threshold 0.7          &  $95.4 \pm 0.3$  &  $74.5 \pm 1.5$  &  $83.5 \pm 1.0$  &  $51.9 \pm 0.9$   &    -----      &    -----      &    -----      &    -----    \\ \hhline{~---------}
&Threshold 0.7 no reset &  $95.5 \pm 0.2$  &  $76.6 \pm 0.9$  &  $85.0 \pm 0.7$  &  $52.7 \pm 0.9$   &    -----      &    -----      &    -----      &    -----    \\ \hhline{~---------}
&Threshold 1.0          &  $94.8 \pm 0.3$  &  $77.8 \pm 1.4$  &  $85.4 \pm 0.9$  &  $52.6 \pm 0.8$   &    -----      &    -----      &    -----      &    -----    \\ \hhline{~---------}
&Threshold 1.0 no reset &  $94.9 \pm 0.2$  &  $\mathbf{80.1 \pm 0.9 }$ &  $\mathbf{86.9 \pm 0.6 }$ &  $53.3 \pm 0.8$   &    -----      &    -----      &    -----      &    -----    \\
\hhline{==========}
    		\end{tabular}
		}
		\end{center}
	\caption{5D sphere, 50 validation.}
	\label{tab:sphere}
\end{table}
